# Supplementary material for: A generalizable saliency map-based interpretation of model outcome
Source: arXiv:2006.09504 source file (2020-06-19)
Supplement: Supplementary file 1 [file appendix.tex]

% \begin{figure*}[!ht]%
% \centering
% \includegraphics[width=0.8\linewidth]{results/reconstructed_region_with_accuracy}%
% \caption{Figures showing the histogram of the reconstructed salient region pixels and the original salient region pixels. The title of the sub-figures show the target accuracy with the reconstructed salient region as well as the original salient region.}%
% \label{fig:overview}%
% \end{figure*}

% \begin{figure*}[!ht]%
% \centering
% \includegraphics[width=0.8\linewidth]{results/saliency_map_comparison_1_2_3}%
% \caption{Saliency map generated for the target-specific images using our approach, RISE~\cite{rise}, GCAM~\cite{grad-cam}, and LIME~\cite{lime}. The header of the input image (leftmost) shows the top predicted class of the model followed by the class accuracy. The header of highlighted images shows the type of approach followed by the measure of deletion/insertion metrics~\cite{rise}.}%
% \label{fig:overview}%
% \end{figure*}
